# Supplementary material for: FinanceComplexQA: Benchmarking Agentic Reasoning on Industrial-grade Financial Documents
Source: arXiv:2607.19238 source file (2026-07-21)
Supplement: Supplementary file 1 [file main.tex]

% Compile: pdflatex main.tex  (run twice for TOC)
% Or include in your paper: \input{appendix-latex/appendix_prompts}

\documentclass[11pt,a4paper]{article}

\usepackage[T1]{fontenc}
\usepackage[utf8]{inputenc}
\usepackage{lmodern}
\usepackage[margin=2.4cm]{geometry}
\usepackage{titlesec}
\usepackage{titletoc}

\input{styles/promptstyle.tex}

% Section styling
\titleformat{\section}{\Large\sffamily\bfseries\color{PromptFrame}}{Appendix \thesection}{0.8em}{}
\titleformat{\subsection}{\large\sffamily\bfseries\color{PromptAccent}}{\thesubsection}{0.6em}{}
\titleformat{\part}{\huge\sffamily\bfseries\color{PromptFrame}}{}{0em}{\centering}

\titlespacing*{\section}{0pt}{1.6em}{0.8em}
\titlespacing*{\subsection}{0pt}{1.2em}{0.5em}

\title{\sffamily\bfseries\color{PromptFrame}FinBench Prompt Templates\\[0.35em]
  {\large\color{PromptMuted}Appendix for Dataset Construction and Document Generation}}
\author{}
\date{}

\begin{document}

\maketitle
\thispagestyle{empty}

\vspace{-0.5em}
\begin{center}
  \color{PromptMuted}\small
  Standalone preview of \texttt{appendix\_prompts.tex}.\\
  Integrate into your paper with \verb|\input{appendix-latex/appendix_prompts}|.
\end{center}

\vspace{1.2em}
\tableofcontents
\newpage

\input{appendix_prompts}

\end{document}
