# Supplementary material for: FinanceComplexQA: Benchmarking Agentic Reasoning on Industrial-grade Financial Documents
Source: arXiv:2607.19238 source file (2026-07-21)
Supplement: Supplementary file 2 [file promptstyle.tex]

% Shared styling for prompt appendix blocks
\RequirePackage{xcolor}
\RequirePackage{tcolorbox}
\tcbuselibrary{breakable,skins,listings}
\RequirePackage{enumitem}
\RequirePackage{booktabs}
\RequirePackage{tabularx}
\RequirePackage{microtype}
\RequirePackage[hidelinks]{hyperref}

\definecolor{PromptFrame}{HTML}{2C3E50}
\definecolor{PromptFill}{HTML}{F8FAFC}
\definecolor{PromptAccent}{HTML}{3B6EA5}
\definecolor{PromptMuted}{HTML}{64748B}
\definecolor{NoteFill}{HTML}{FFF8E7}
\definecolor{NoteFrame}{HTML}{D4A017}

\newtcolorbox{promptmeta}[1]{
  enhanced,
  breakable,
  colback=PromptFill,
  colframe=PromptAccent,
  arc=2.5mm,
  boxrule=0.6pt,
  left=10pt,
  right=10pt,
  top=8pt,
  bottom=8pt,
  title={#1},
  fonttitle=\bfseries\sffamily,
  coltitle=white,
  attach boxed title to top left={yshift=-2.5mm, xshift=5mm},
  boxed title style={
    colback=PromptAccent,
    arc=1.5mm,
    boxrule=0pt,
    top=2pt,
    bottom=2pt,
    left=6pt,
    right=6pt
  }
}

\newtcolorbox{promptnote}{
  enhanced,
  breakable,
  colback=NoteFill,
  colframe=NoteFrame,
  arc=2mm,
  boxrule=0.5pt,
  left=10pt,
  right=10pt,
  top=6pt,
  bottom=6pt,
  fontupper=\small
}

\NewTCBListing{promptbody}{ !O{} }{
  enhanced,
  breakable,
  colback=PromptFill,
  colframe=PromptFrame,
  arc=2mm,
  boxrule=0.4pt,
  left=8pt,
  right=8pt,
  top=6pt,
  bottom=6pt,
  listing only,
  listing options={
    basicstyle=\small\ttfamily,
    breaklines=true,
    breakatwhitespace=false,
    columns=fullflexible,
    keepspaces=true,
    showstringspaces=false,
    aboveskip=0pt,
    belowskip=0pt
  },
  #1
}
